# Supplementary material for: Phase-dependent epitaxy for antimonene growth on silver substrate
Source: arXiv:2112.07119 source file (2021-12-14)
Supplement: Supplementary file 1 [file si.pdf]

# Supplementary Information: Phase-dependent epitaxy for antimonene growth on silver substrate

Kai Liu,[1,*] Keke Bai,[1,*] Jing Wang,[1,†] Juntao Song,[1] and Ying Liu[1,2]

[1]*Department of Physics and Hebei Advanced Thin Film Laboratory, Hebei Normal University, Shijiazhuang 050024, Hebei, China.*

[2]*National Key Laboratory for Materials Simulation and Design, Beijing 100083, China*

(Dated: December 14, 2021)

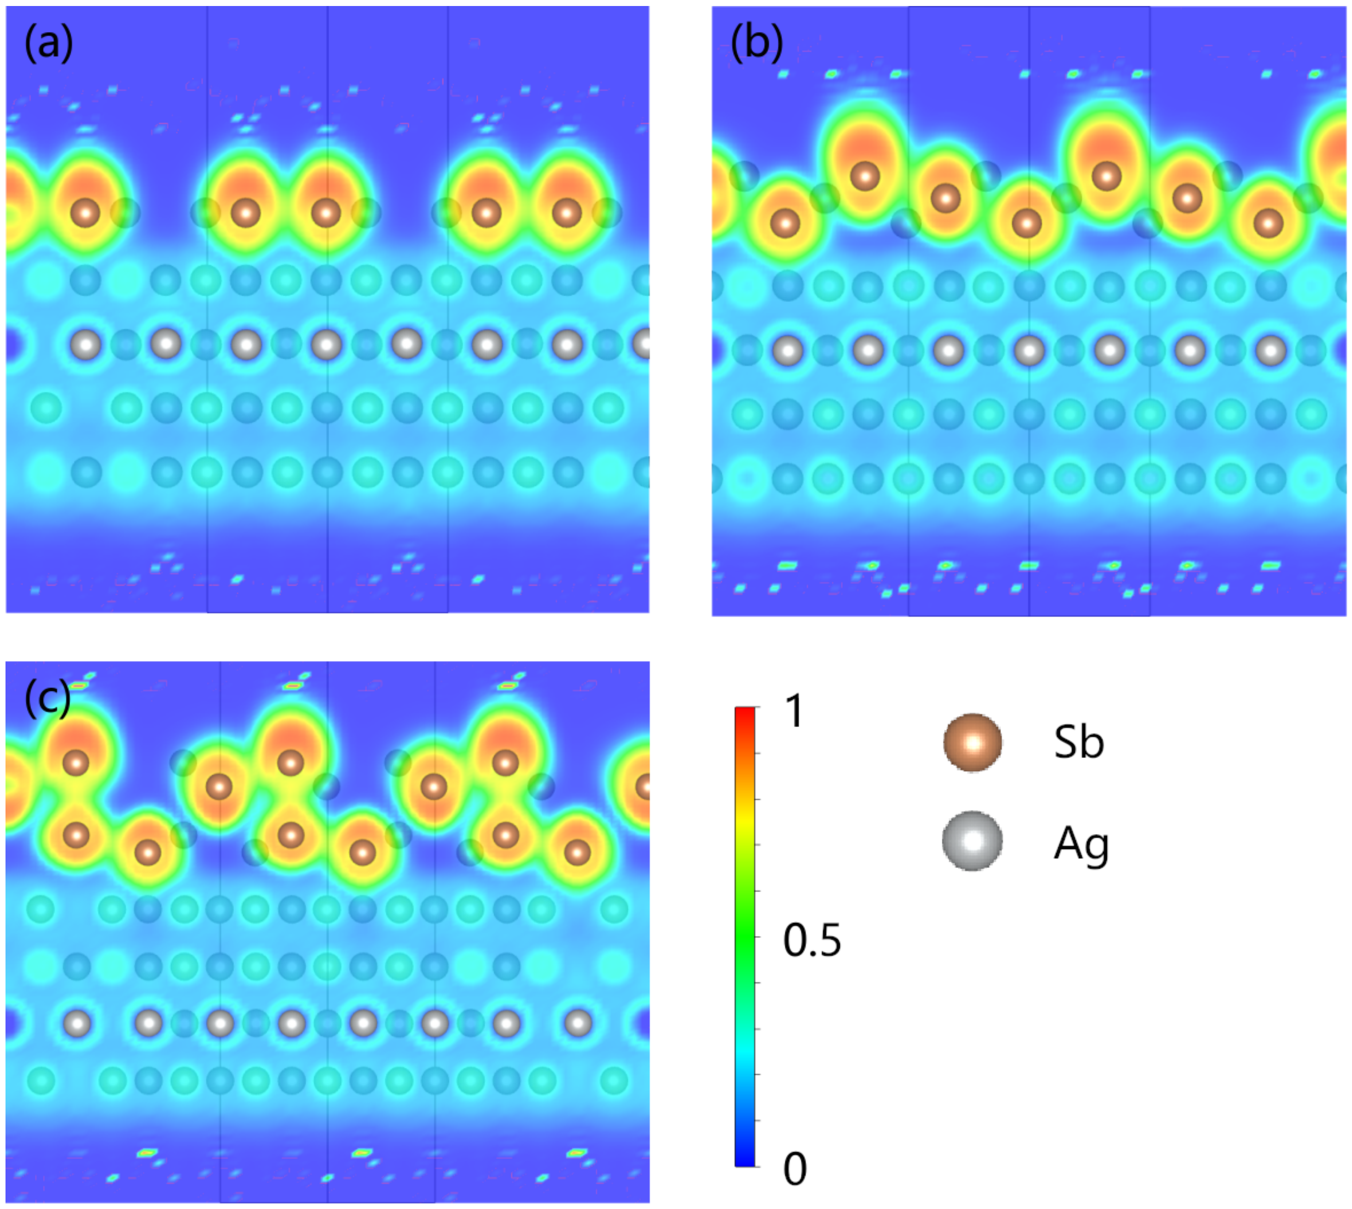


FIG. S1. 2D contour plot of the electron localization function (ELF) of Sb atoms on a pure Ag (111) substrate at $C_{Sb}$ = (a) 2/3, (b) 3/3, and (c) 4/3 along the cut of the Miller index (110). The minimum ELF value is 0.0 (blue) and the maximum value is 1.0 (red). The brown and silver balls represent Sb and Ag, respectively.

---

* These authors equally contribute to this work.

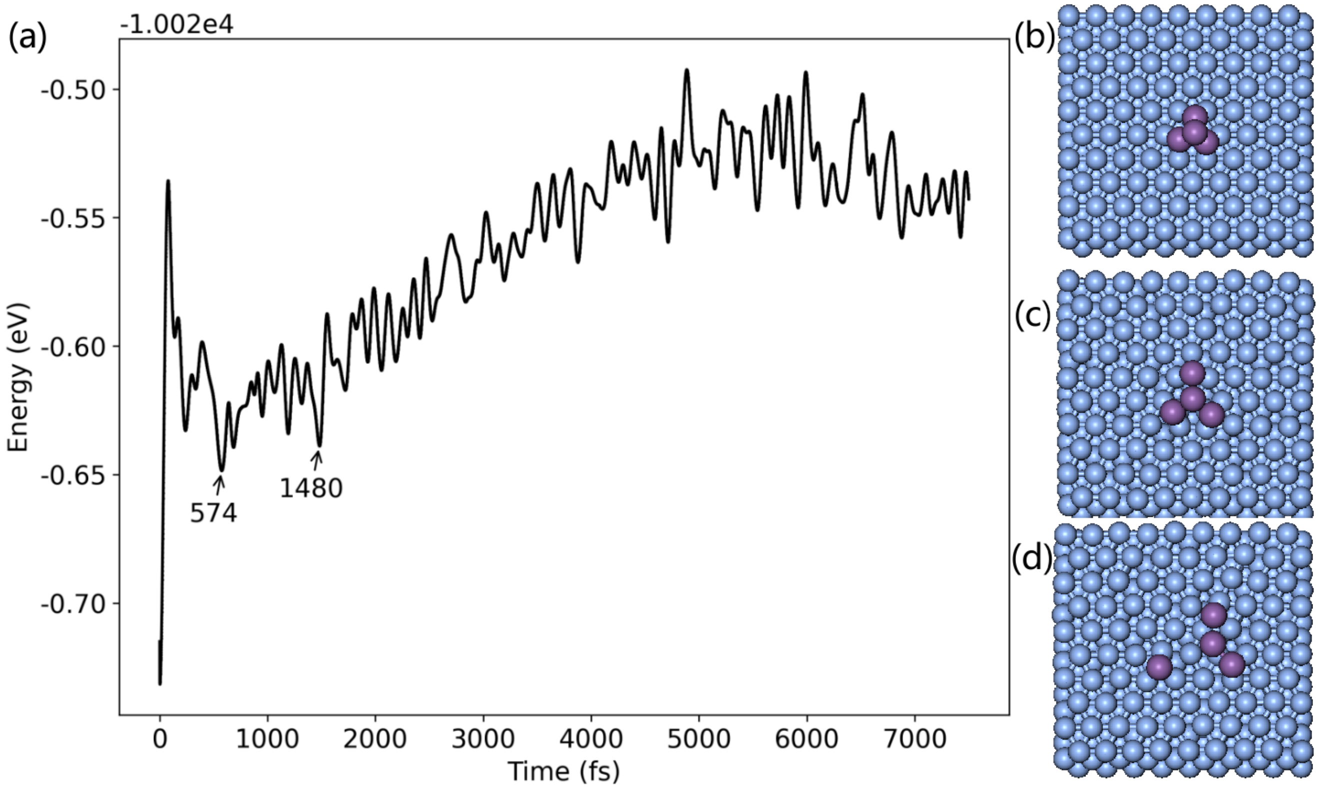


FIG. S2. (a) Total energy of system as a function of time from the AIMD simulation for one $Sb_4$ clusters on pure Ag(111) surface at 300K and zero pressure; System structures at (b) 0 fs (initial configuration), (c) 574 fs ($Sb_4$ cluster began to collapse to planar configuration, it's configuration with the lowest energy of planar ones), (d) 1480 fs (all Sb atoms sit in a plane, and cluster was departed into two parts) are listed at right, respectively.

† jwang@hebtu.edu.cn

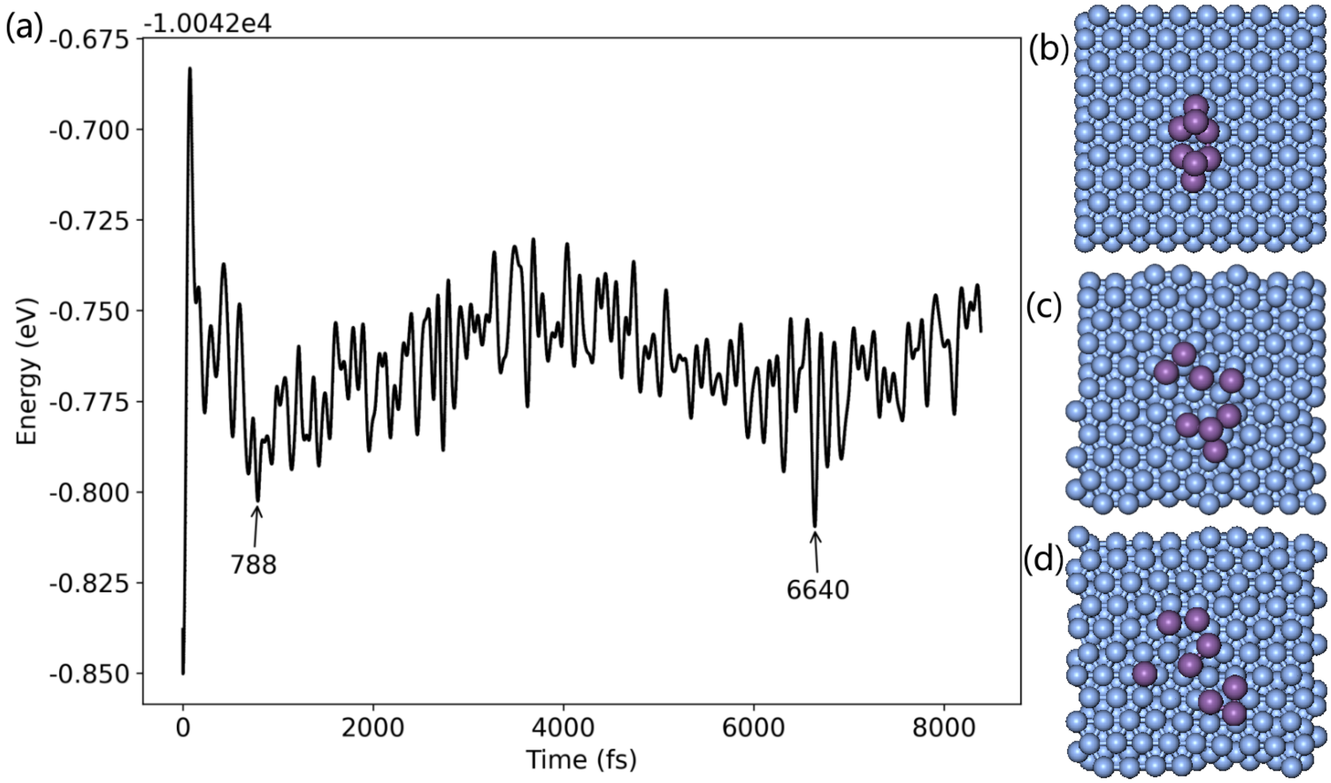


FIG. S3. (a) Total energy of system as a function of time from the AIMD simulation for two $Sb_4$ clusters on pure Ag(111) surface at 300K and zero pressure; System structures at (b) 0 fs (initial configuration), (c) 788 fs (one of $Sb_4$ clusters collapse to planar configuration), (d) 6640 fs (the configuration with the second-lowest energy) are listed at right, respectively.

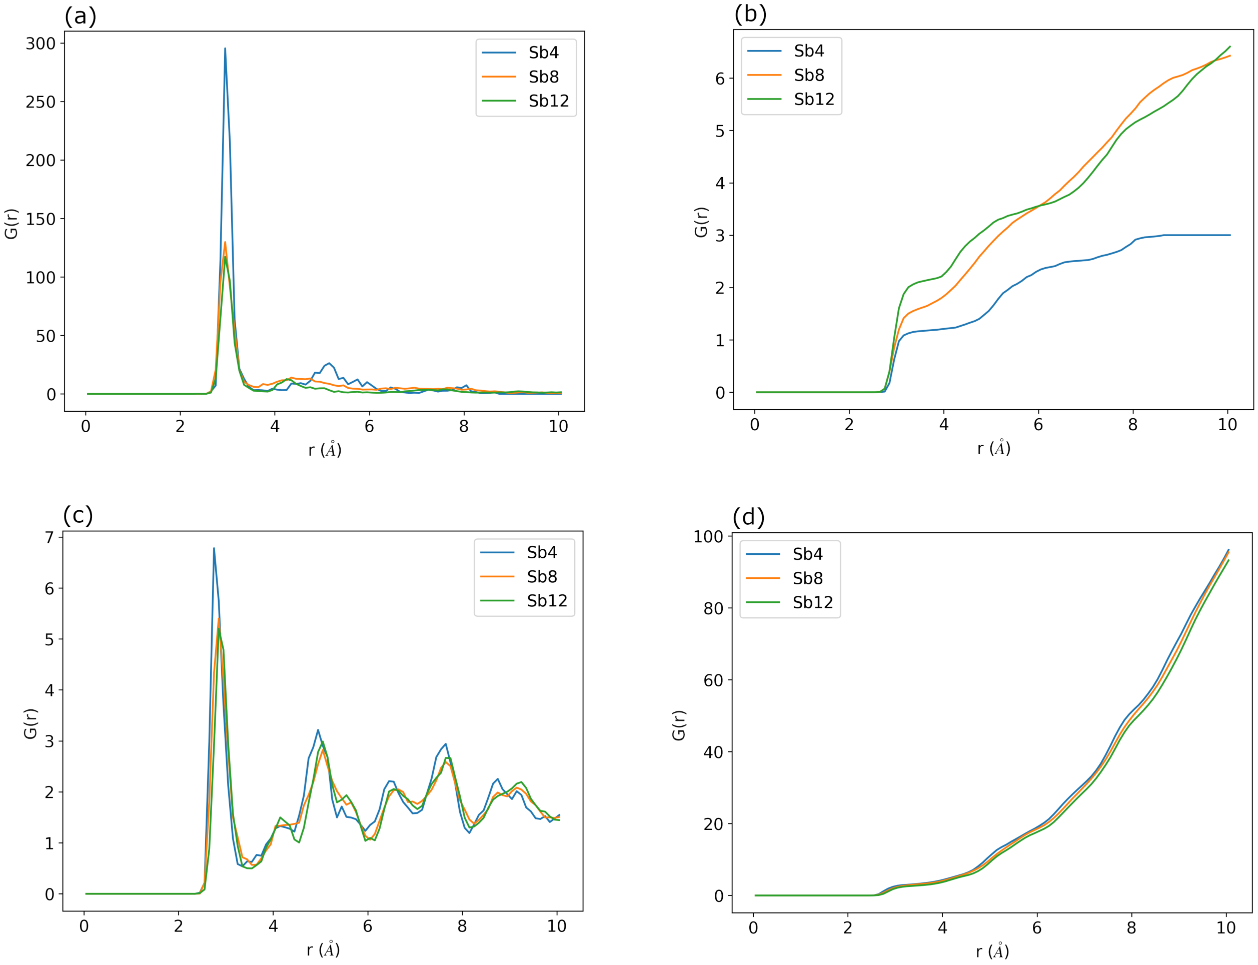


FIG. S4. (a) and (c) are the radial distribution function for Sb-Sb and Sb-Ag, respectively. (b) and (d) are integration curve of (a) and (c).

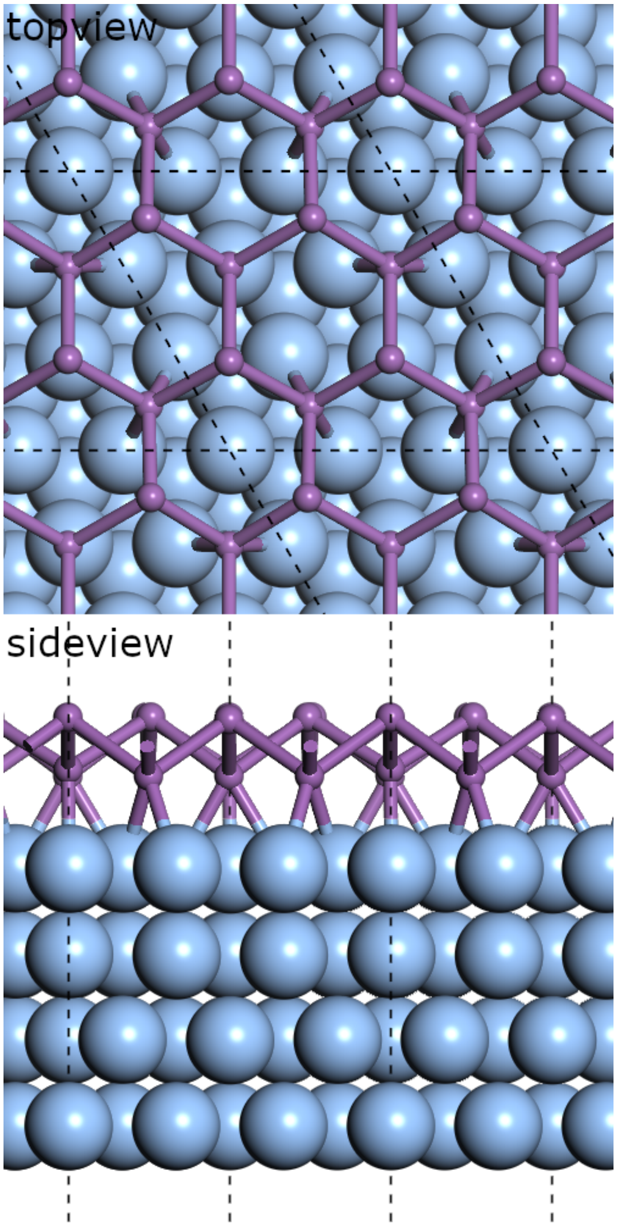


FIG. S5. Top and side views of configuration at $C_{Sb}$ = 8/9 on pure Ag(111) surface. Antimony atoms formed a buckled honeycomb lattice, which is exactly the $\beta$ phase antimonene. This configuration is the sub-stable one at $C_{Sb}$ = 8/9, the formation energy of it is 0.035 eV/atom higher than that of the most stable configuration.
